# Supplementary material for: Free-Editor: Zero-shot Text-driven 3D Scene Editing
Source: arXiv:2312.13663 source file (2024-07-14)
Supplement: Supplementary file 1 [file X_suppl.tex]

\section{Overview}
The overview of this supplementary is as follows:
\begin{itemize}
    \item In Section~\ref{sec:background}, we provide additional background details about diffusion-guided editing. 
    \item Section~\ref{sec:experimental_settings} contains the details of the data generation process using target captions, architecture details, as well as training and inference. In Algorithm~\ref{alg:free_editor}, we summarize our proposed method.  
    \item In Section~\ref{sec:user_study}, we provide the details of the user study.
    \item Additional qualitative and quantitative results are in Section~\ref{sec:add_results}.  
    \item Section~\ref{sec:need_for_free_editor} contains some discussions on the uniqueness of the Free-Editor.
    % \item \emph{We have added the video results with the PDF file. Due to the 100 MB size limit of ECCV, we needed to heavily compress some of the video samples. The video quality may be poor for those samples.} 
\end{itemize}

\section{Background}\label{sec:background}

\noindent \textbf{Text-to-Image (T2I) Diffusion Model.} The Stable Diffusion (SD) model~\cite{rombach2022high} operates within the latent space of an autoencoder $\mathcal{D}(\mathcal{E}(\cdot))$, specifically VQ-GAN \cite{esser2021taming} or VQ-VAE \cite{van2017neural}. Here, $\mathcal{E}$ denotes the encoder compressing an RGB image $x$ into a low-resolution latent $z = \mathcal{E}(x)$, recoverable using the decoder $x \sim \mathcal{D}(z)$. The diffusion forward process includes iterative addition of Gaussian noise to the signal $z$ as follows:
\begin{equation}
q(z_t|z_{t-1}) = \mathcal{N}(z_t; \sqrt{1-\beta_t}z_{t-1}, \beta_t I); t = 1,2\ldots T,
\end{equation}
where $q(z_t|z_{t-1})$ represents the conditional density of $z_t$ given $z_{t-1}$, and ${\beta_t}{t=1}^{T}$ are hyperparameters.
$T$ is selected sufficiently large to ensure $z_T \sim \mathcal{N}(0,I)$. Subsequently, a U-Net~\cite{ronneberger2015u} comprising convolutional, self, and cross attentional blocks with parameters $\theta$ undergoes training for the backward process, i.e., denoising, using the objective function:
%\vspace{-0.5em}
\begin{equation}
\min _\theta E_{z_0, \varepsilon \sim N(0, I), t \sim \text { Uniform }(1, T)}\left\|\varepsilon-\varepsilon_\theta\left(z_t, t, p \right)\right\|_2^2,
\end{equation}
where $p$ stands for the embedding of prompt $p = \mathcal{C}(\mathcal{P};\phi)$ and $\varepsilon\theta$ represents the model-predicted noise at time $t$. During inference, deterministic DDIM sampling~\cite{ddim} is applied to convert a random noise $z_T$ into a clean latent $z_0$. In our work, we use InstructPix2Pix as the T2I model which is also a latent diffusion-based method specialized for image editing. 

\noindent \textbf{A Literature Study on Diffusion-based 2D Image Editing.} Text-guided image synthesis has garnered substantial attention within the generative model domain~\cite{abdal2021clip2stylegan, abdal2021styleflow, avrahami2022blended, zhang2021cross, geng2023hiclip, oh2001image, xu2018attngan}. Recent advancements in diffusion models \cite{sohl2015deep,song2020denoising} have presented innovative approaches, yielding impressive outcomes~\cite{ramesh2022hierarchical,rombach2022high,saharia2022photorealistic}. With significant enhancements in this domain, the focus has been shifted from training extensive text-to-image models from scratch to leveraging open-source pre-trained models for prompt-guided image manipulation ~\cite{gal2023an,hertz2022prompt,kawar2023imagic,liu2023more}. These text-driven editing techniques serve diverse purposes like image editing, style transfer, and generator domain adaptation~\cite{10484324, kwon2023diffusion, ruiz2023dreambooth, han2023svdiff, zhang2023adding, yang2023zero}.

\begin{algorithm}[t]
\caption{Working Principle of \textsc{Free-Editor}}

\begin{algorithmic}[1]
\State \textbf{Input:} T2I Edited Starting View Image $\hat{I}_0$, Multi-view non-edited Source Images $\{I_m, P_m\}_{m=1}^{M}$,  Points coordinate in target view $\Mat{p}_{t} \rightarrow (N_{\text{rays}}, N_P, 3)$, Number of target rays $N_{\text{rays}}$, Number of sampled points along each ray $N_P$, 2D Image Encoder $T$ \\
\State \textbf{Notations:} 
% \State $\Mat{v_{t}} \rightarrow \text{view direction of each point} (N_{\text{rays}}, P, D_2)$
\State $\hat{f}_0 = \bm{T}(\hat{I}_0)$ \Comment{flattened patch tokens in edited starting view $(1, N_{\text{patch}}, C)$}
\State $\bm{f}_m = \bm{T}(\hat{I}_m); m = 1, \ldots M$ \Comment{flattened patch tokens in starting view $(M, N_{\text{patch}}, C)$}
\State $W_{Q}, W_{K}, W_{V}, W_{\text{rgb}} \rightarrow \text{functions that parameterize MLP layers}$

\State \textbf{Edit Transformer:} 
    % \State $X_{o} = f_{P}(\Mat{{f}_m})$ 
    \State $\Mat{Q} = W_{Q}(\hat{f}_0)$ \Comment{For Self-view attention}
    
    \State $\Mat{K} = W_{K}(\hat{f}_0)$
    \State $\Mat{V} = W_{V}(\hat{f}_0)$
    \State $\Mat{A} = \operatorname{matmul}(\Mat{Q}, \Mat{K}^{T}) / \sqrt{D}$
    \State $\Mat{A} = \operatorname{softmax}(\Mat{A}, \operatorname{dim}=-1)$                  
    \State $\hat{f}_0 = \operatorname{matmul}(\Mat{A}, \Mat{V})$

\For{$1 \leq m \leq M$}  \Comment{For Cross-view attention}
    \State $\Mat{Q} = W_{Q}({f}_m)$
    \State $\Mat{K} = W_{K}(\hat{f}_0)$
    \State $\Mat{V} = W_{V}(\hat{f}_0)$
    \State $\Mat{A} = \operatorname{matmul}(\Mat{Q}, \Mat{K}^{T}) / \sqrt{D}$
    \State $\Mat{A} = \operatorname{softmax}(\Mat{A}, \operatorname{dim}=-1)$
    \State $\Mat{{f}_m} = \operatorname{matmul}(\Mat{A}, \Mat{V})$
\EndFor

\For {$1 \leq m \leq M$}
\For {$0 \leq i \leq (N_{\text{rays}} \times P)$} \Comment{projected points feature along target ray $(N_{\text{rays}}, N_P, D)$}
    \State $\Mat{e}_t^{i,m} = \operatorname{interp.}(\operatorname{proj.}(\operatorname{modulation}(\Mat{p}_t^i), \Mat{X}_m))$
\EndFor
\EndFor

\State \textbf{Epipolar Transformer:} 

\For {$0 \leq i \leq (N_{\text{rays}} \times P)$} 
\State $\Mat{e}_t^i \rightarrow$ Output of Eq.~\ref{eq:epi_final}
\EndFor

\State \textbf{Ray Transformer:} 

\For {$0 \leq i \leq N_{\text{rays}}$}  \Comment{Ray attention}
    % \State $X_{o} = f_{P}(\Mat{X_{0}})$
    \State $\Mat{Q} = W_{Q}(\Mat{e}_t^i)$
    \State $\Mat{K} = W_{K}(\Mat{e}_t^i)$
    \State $\Mat{V} = W_{V}(\Mat{e}_t^i)$
    \State $\Mat{A} = \operatorname{matmul}(\Mat{Q}, \Mat{K}^{T}) / \sqrt{D}$
    \State $\Mat{A} = \operatorname{softmax}(\Mat{A}, \operatorname{dim}=-1)$
    \State $\Mat{e}_t^i = \operatorname{matmul}(\Mat{A}, \Mat{V})$ 
\EndFor

\State $\text{Get the Predicted RGB Image}, \tilde{I}_t = W_{\text{rgb}}(\operatorname{mean}_{i=1}^{N_P}(\Mat{e}_t^i))$
\State Calculate Total Loss, $\mathcal{L}_{tot}$
\State Backpropagate the loss and update the model except for 2D encoder $T(.)$
\end{algorithmic}
\label{alg:free_editor}
\end{algorithm}

\begin{figure*}[t]
%\begin{center}
\centering
%\hspace{-5mm}
%\begin{minipage}{0.35\textwidth}
    \includegraphics[width=1\linewidth]{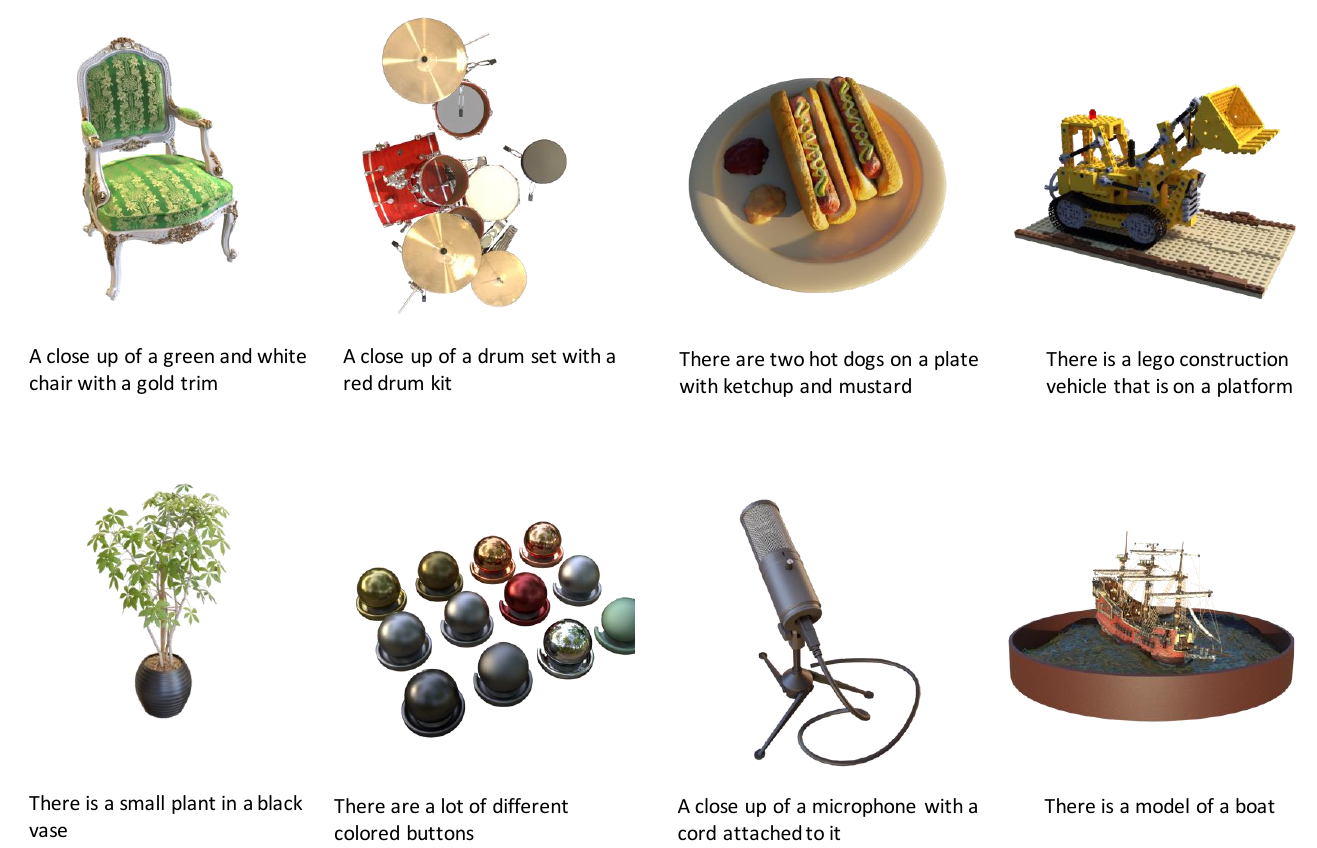}
%    \end{center}
    %\vspace{-5mm}
    \caption{ \textbf{BLIP Generated Input Captions.} These captions will later be converted to different target editing prompts to edit the starting views. We store all the editing prompts in a separate file and use that during training.}
 
\label{fig:blip_gen_captions}
% %\vspace{-2mm}
\end{figure*}

% \paragraph{Text-to-3D Scene Editing Method, InstructNeRF2NeRF.} operates by repeatedly updating the training dataset images using a diffusion model and then training the NeRF on these modified images to maintain a consistent 3D representation. This iterative approach allows the gradual integration of the diffusion priors into the 3D scene, enabling substantial edits. The use of an image-conditioned diffusion model (InstructPix2Pix) helps preserve the original scene's structure and identity. More details are in their original paper. 

% , NerfStudio~\cite{tancik2023nerfstudio}, NeRF-Art~\cite{wang2023nerf}, Spaces~\cite{flynn2019deepview}, and IBRNet-collect~\cite{wang2021ibrnet}

\section{Experimental Settings}\label{sec:experimental_settings}
\subsection{Data Generation}\label{sec:data_gen}
We train on around 1500 scenes from different datasets\footnote{We also consider scenes from a recent 3D dataset, Objaverse~\cite{deitke2023objaverse}}.  For example, we take around 1000 object-centric renderings of common household items from Google Scanned Objects~\cite{downs2022google}, 100 indoor and outdoor scenes from Spaces~\cite{flynn2019deepview}, 67 scenes from IBRNet-collect~\cite{wang2021ibrnet}, 18 scenes from NerfStudio~\cite{tancik2023nerfstudio}, 80 scenes from RealEsta-te10K~\cite{zhou2018stereo}, etc. For each scene, we randomly select a starting view image and edit it using a diffusion model. Now to edit this image, we need to use a text prompt. To generate this text prompt, we need to first generate the image caption of the starting view using a BLIP model. We show some of the BLIP-generated input captions in Figure~\ref{fig:blip_gen_captions}. After obtaining the initial captions for each scene, we utilized the GPT model to generate target captions. Our process involved requesting GPT to provide lists featuring 100 renowned painters, 100 paintings, and 50 painting schools. These generated elements from GPT were then merged with the initial captions using a predefined structure to produce target captions emphasizing style transfer. To address other editing requirements, we directed GPT to perform actions such as adding, removing, or replacing words within the initial captions. For example, we may have painting styles such as  ["Baroque", "Realism", "Impressionism","Op Art", "Fauvism", ..... ....., "Tonalism","Ashcan School", "Rococo", "Symbolism", "Outsider Art"]. On the other hand, different painter styles could be ["Leonardo da Vinci", "Vincent van Gogh", "Sam Francis", "Max Ernst", "Henri Matisse", "Eva Hesse", .... ...., "Carl Andre", "Cy Twombly"]. We also consider different colors such as ["pink", "red", "orange", ... , "white","purple","green","blue", "silver", "gold", 'bronze']. We randomly choose an editing style and generate a target caption from the source caption.

% We divide these editing styles into train and test sets. From the train set,During inference, we use the editing styles form the test set.

For editing an image, we use IP2P model where one can specify the classifier-free guidance weights, $C_g$, to control the specific amount of change in a given input image. Here, $C_g$ can vary from scene to scene. For example, we use a value of 7 for \emph{Bear} and 8.5 for the \emph{human} scene. In our experiments, we consider a range of values for $C_g$, i.e. $C_g \in [6.5, 12.5]$. We follow the GitHub Repository~\url{https://github.com/huggingface/diffusers} for IP2P implementations.
\subsection{Architecture Details}
To extract features from the edited and un-edited source views, we adopt a pre-trained ResNet50 ImageNet encoder. We also tried the DinoV2 encoder~\cite{oquab2023dinov2} for feature extration. After extracting the feature maps, we feed them to the Edit Transformer and finally aggregate the features along the epipolar line using an Epipolar Transformer.
\subsubsection{Edit Transformer}
Within each edit transformer block, there exist multi-headed self and cross-attention layers. In our experiments, we use 8 heads for each attention layer. Outputs from these attention layers proceed to respective feedforward blocks employing Rectified Linear Unit (RELU) activation and a hidden dimension of $256$. A residual connection connects pre-normalized inputs (LayerNorm) to outputs at every layer. To save computation for high-resolution images, we propose utilizing 8$\times$ downsampled CNN features, pooling them into fixed-size 2D grids (in our case, a 7$\times$7 grid) for each view. This design is resolution-agnostic, enabling attention in a patch-wise manner regardless of input resolution.

\begin{figure*}[!t]
%\begin{center}
\centering
%\hspace{-5mm}
%\begin{minipage}{0.35\textwidth}
    \includegraphics[width=1\linewidth]{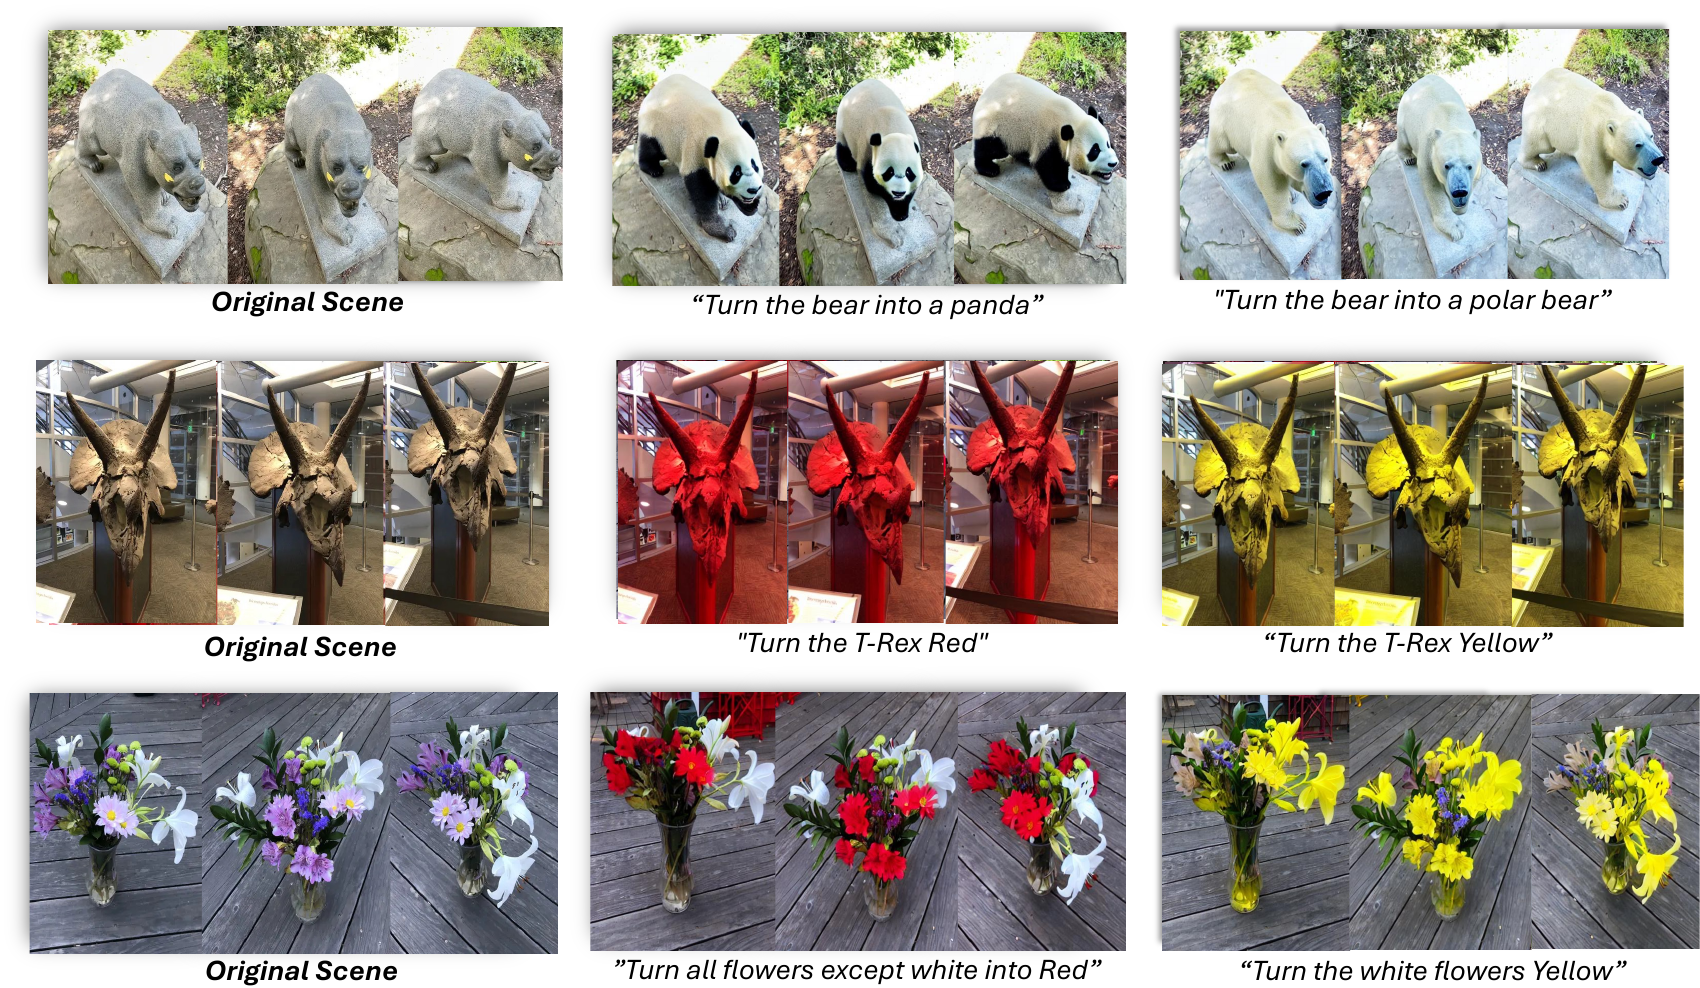}

    \includegraphics[width=1\linewidth]{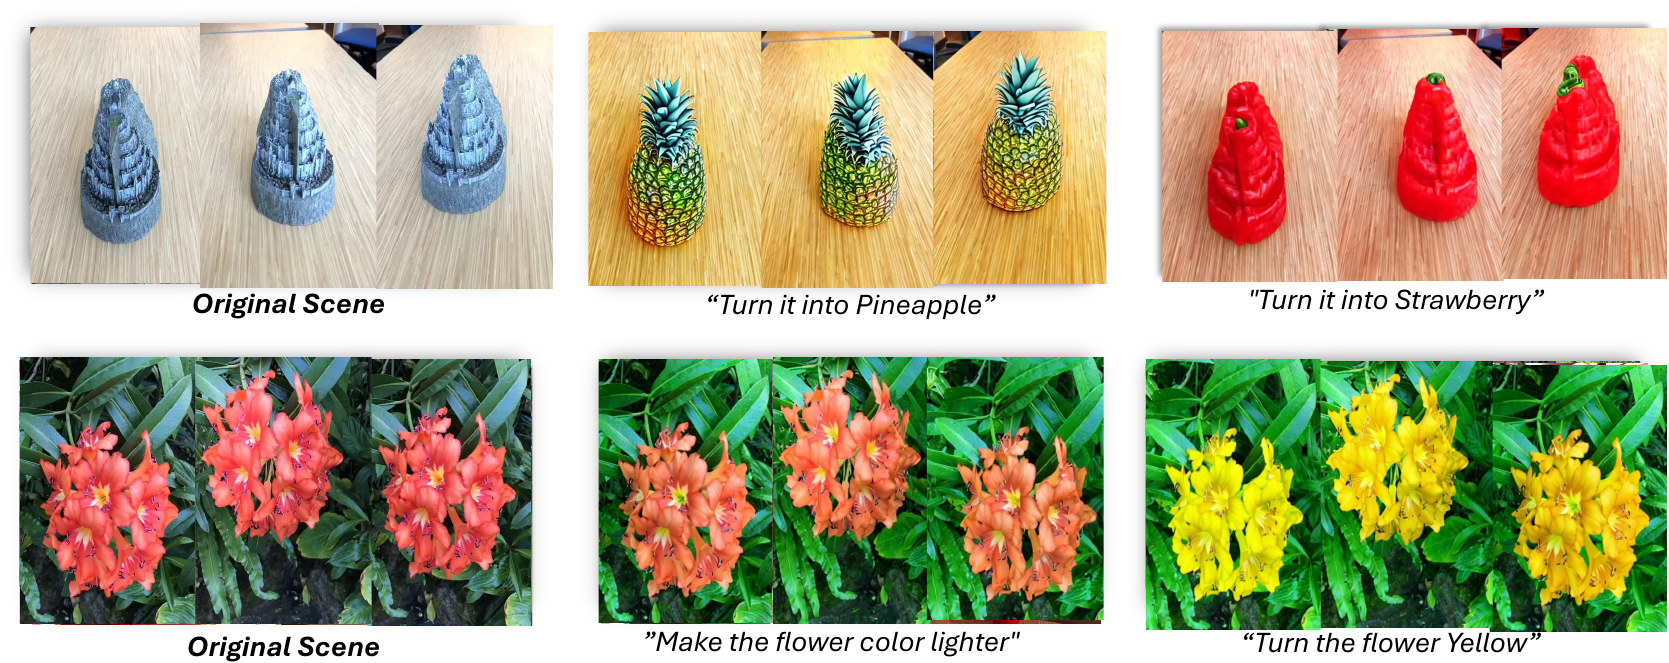}
    
%    \end{center}
    %\vspace{-2mm}
    \caption{ \textbf{Text-driven 3D scene editing.} Illustration of text-driven 3D scene editing using our proposed method across various target poses. }
 
\label{fig:text_to_3D_1}
% %\vspace{-2mm}
\end{figure*}

\subsubsection{Epipolar Transformer}
We follow GNPR~\cite{suhail2022generalizable} to build the epipolar transformer, consisting of 6 transformer blocks. This transformer aggregates information along each epipolar line,
resulting in per-reference (unedited source) view features.
Let us consider $N_{\text{rays}}$ as the number of target rays and $N_P$ is the number of sampled points along each ray. For each of these sampled points, we have  $e_1 = \{e_1^p \mid 1 \le p \le N_e\}$ which we get from the Edit Transformer,
concatenated with positional encodings $r_k^p,\, d^p,\, c_k$. Here, $N_e$ is the number of sampled points along the epipolar line in each source-view image.
We refer to the features corresponding to view $k$ in the set $e_1^p$ as $e_1^{k, p}$.
The transformer is repeated for each view, therefore operating along the sequence of
$N_e$ epipolar line samples.
Formally, we first compute
\begin{align}
  e_2^{k} = E_1\left(
  \Big\{ r^0 \Big\} \bigcup
  \left\{\left[e_1^{k,p} \;\Big\|\; r_k^p \;\Big\|\; d^p \;\Big\|\; c_k \right]
  \;\Big|\; 1 \le p \le N_e\right\}\right),
\end{align}
for $1 \le k \le K$, where $r^0$ is a special token to represent the target ray. Here, $E_1$ is the first segment of the Epipolar transformer, consisting of 4 transformer blocks.
We then apply a learned weighted sum along the $N_e$ epipolar line samples as follows,
\begin{align}
  \label{eq:alpha}
  \alpha_{k}^{p} &= \frac{\exp \left(W_{1} \left[e_2^{k,0} \;\Big\|\; e_2^{k, p}\right] \right)}
  { \sum\limits_{p'=1}^{N_e} \exp \left(W_{1} \left[e_2^{k,0} \;\Big\|\; e_2^{k, p'}\right] \right)}, \\
  e_{2'}^k &= \sum_{p=1}^{N_e} \alpha_{k}^{p} e_2^{k, p},
\end{align}
for $1 \le k \le M$,
resulting in a feature vector per view $k$,
where $W_1$ are learnable weights and 
$e_2^{k,0}$ is the output corresponding to the target ray token.

Dimension-wise, this stage takes a $(N_{\text{rays}}, N_P, M, N_e, D)$ tensor 
and returns a $(N_{\text{rays}}, N_P,M, D)$  tensor. After this, we compute
\begin{align}
  e_3^{k} = E_3\left(
  \Big\{ r^0 \Big\} \bigcup \left\{\left[e_{2'}^{k} \;\Big\|\; c_k \right]
  \;\Big|\; 1 \le k \le M\right\}\right).
\end{align}
Similarly to the previous stage, we compute the blending weights
\begin{align}
  \label{eq:beta}
  \beta_{k} &= \frac{\exp \left(W_{2} \left[e_3^0 \;\Big\|\; e_3^{k}\right] \right)}
  { \sum\limits_{k'=1}^M \exp \left(W_{2} \left[e_3^{0} \;\Big\|\; e_3^{k}\right] \right)}, \\
  e_{t} &=  \sum\limits_{k=1}^M \beta_k e_3^{k}, \label{eq:epi_final}
\end{align}
here $W_{2}$ is the learnable weights. Finally, we obtain a $(N_{\text{rays}}, N_P, D)$ tensor that will be fed to the Ray Transformer.

\begin{table*}[!t]
    \caption{\textbf{Comparison of \textsc{Free-Editor} against SOTA generalizable NeRF models} for single scene rendering on the real forward-facing LLFF Dataset (scene-wise). The evaluation metrics are PSNR (higher is better), SSIM~\cite{wang2004image} (higher is better), and LPIPS~\cite{zhang2018unreasonable} (lower is better) metrics.}
    %\vspace{-2.5mm}
    \begin{center}
        \begin{threeparttable}
        \scalebox{0.9}{
            \begin{tabular}{l|cccccccccc}
            \toprule
            & \multicolumn{8}{c}{PSNR$\uparrow$} \\
            \cmidrule{2-9}
            &  Fern & Flower & Fortress & Horns & Leaves & Orchids & Room & T-Rex \\
            \midrule
            pixelNeRF~\cite{yu2021pixelnerf} & 12.40 & 10.00 & 14.07 & 11.07 & \phantom{0}9.85 & \phantom{0}9.62 & 11.75 & 10.55 \\
            IBRNet~\cite{wang2021ibrnet} & 23.84 & 26.67 & 30.00 & 26.48 & 20.19 & 19.34 & \textbf{29.94} & \textbf{24.57} \\
            MVSNeRF~\cite{chen2021mvsnerf} & 21.15 & 24.74 & 26.03 & 23.57 & 17.51 & 17.85 & 26.95 & 23.20 \\
            GeoNeRF~\cite{johari2022geonerf} & \textbf{24.61} & \textbf{28.12} & \textbf{30.49} & \textbf{26.96} & \textbf{20.58} & \textbf{20.24} & 28.74 & 23.75 \\
            \midrule
            \textsc{Free-Editor} & 23.18 & 26.87 & 28.10 & 24.93 & 20.06 & 19.49 & 27.14 & 21.72 \\
            \bottomrule
            \end{tabular}}
        \end{threeparttable}
        \begin{threeparttable}
            \scalebox{0.9}{
            \begin{tabular}{l|cccccccccc}
            \toprule
            & \multicolumn{8}{c}{SSIM$\uparrow$} \\
            \cmidrule{2-9}
            &  Fern & Flower & Fortress & Horns & Leaves & Orchids & Room & T-Rex \\
            \midrule
            pixelNeRF~\cite{yu2021pixelnerf} & 0.531 & 0.433 & 0.674 & 0.516 & 0.268 & 0.317 & 0.691 & 0.458 \\
            IBRNet~\cite{wang2021ibrnet} & 0.772 & 0.856 & 0.883 & 0.869 & 0.719 & 0.633 & 0.946 & 0.861 \\
            MVSNeRF~\cite{chen2021mvsnerf} & 0.638 & \textbf{0.888} & 0.872 & 0.868 & 0.667 & 0.657 & \textbf{0.951} & 0.868 \\
            GeoNeRF~\cite{johari2022geonerf} & \textbf{0.811} & 0.885 & \textbf{0.898} & \textbf{0.901} & 0.741 & \textbf{0.666} & 0.935 & \textbf{0.877} \\
            \midrule
            \textsc{Free-Editor} & 0.716 & 0.795 & 0.822 & 0.873 & \textbf{0.743} & 0.621 & 0.874 & 0.825 \\
            \bottomrule
            \end{tabular}}
        \end{threeparttable}
        \begin{threeparttable}
            \scalebox{0.9}{
            \begin{tabular}{l|cccccccccc}
            \toprule
            & \multicolumn{8}{c}{LPIPS$\downarrow$} \\
            \cmidrule{2-9}
            &  Fern & Flower & Fortress & Horns & Leaves & Orchids & Room & T-Rex \\
            \midrule
            pixelNeRF~\cite{yu2021pixelnerf} & 0.650 & 0.708 & 0.608 & 0.705 & 0.695 & 0.721 & 0.611 & 0.667 \\
            IBRNet~\cite{wang2021ibrnet} & 0.246 & 0.164 & 0.153 & 0.177 & 0.230 & 0.287 & 0.153 & 0.230 \\
            MVSNeRF~\cite{chen2021mvsnerf} & 0.238 & 0.196 & 0.208 & 0.237 & 0.313 & 0.274 & 0.172 & \textbf{0.184} \\
            GeoNeRF~\cite{johari2022geonerf} & \textbf{0.202} & \textbf{0.133} & \textbf{0.123} & \textbf{0.140} & \textbf{0.222} & \textbf{0.256} & \textbf{0.150} & 0.212 \\
            \midrule
            \textsc{Free-Editor} & 0.234 & 0.208 & 0.126 & 0.182 & 0.263 & 0.271 & 0.191 & 0.217 \\
            \bottomrule
            \end{tabular}}
        \end{threeparttable}
    \end{center}
        % %\vspace{-3ex}

    % %\vspace{3ex}
    \label{table:llfe_original}
\end{table*}

% \begin{table*}[!t]
%     \begin{center}
%             \scalebox{0.8}{
%             \begin{tabular}{l|cccccccccc}
%             \toprule
%             & \multicolumn{8}{c}{PSNR$\uparrow$} \\
%             \cmidrule{2-9}
%             &  Fern & Flower & Fortress & Horns & Leaves & Orchids & Room & T-Rex \\
%             \midrule
%             IBRNet~\cite{wang2021ibrnet} & 18.25 & 20.10 & 21.33 & 20.28 & 14.23 & 12.62 & 21.24 & 19.41 \\
%             GeoNeRF~\cite{johari2022geonerf} & 20.54 & 23.18 & 24.14 & 22.04 & 16.36 & 15.52 & 22.94 & 19.85 \\
%             \midrule
%             \textsc{Free-Editor} & \textbf{22.84} & \textbf{24.15} & \textbf{21.02} & \textbf{23.64} & \textbf{20.19} & \textbf{19.48} & \textbf{24.92} & \textbf{20.46} \\
%             \bottomrule
%             \end{tabular}}
%     \end{center}
%     % %\vspace{-5.5ex}
% \end{table*}
\begin{table*}[!t]
    \caption{\textbf{Comparison of \textsc{Free-Editor} against SOTA for edited LLFF dataset, denoted by LLFF-E}. The performance of SOTA methods drops significantly in this case.}
    %\vspace{-2mm}
    \begin{center}
            \scalebox{0.9}{
            \begin{tabular}{l|cccccccccc}
            \toprule
            & \multicolumn{8}{c}{PSNR$\uparrow$} \\
            \cmidrule{2-9}
            &  Fern & Flower & Fortress & Horns & Leaves & Orchids & Room & T-Rex \\
            \midrule
            IBRNet~\cite{wang2021ibrnet} & 19.25 & 20.10 & 21.33 & 19.28 & 15.23 & 14.62 & 22.24 & 18.41 \\
            GeoNeRF~\cite{johari2022geonerf} & 19.54 & 21.18 & 19.14 & 20.04 & 16.36 & 15.52 & 20.94 & 16.85 \\
            \midrule
            \textsc{Free-Editor} & \textbf{22.84} & \textbf{24.15} & \textbf{21.02} & \textbf{23.64} & \textbf{20.19} & \textbf{19.48} & \textbf{24.92} & \textbf{20.46} \\
            \bottomrule
            \end{tabular}}
            
        \scalebox{0.9}{
            \begin{tabular}{l|cccccccccc}
            \toprule
            & \multicolumn{8}{c}{SSIM$\uparrow$} \\
            \cmidrule{2-9}
            &  Fern & Flower & Fortress & Horns & Leaves & Orchids & Room & T-Rex \\
            \midrule
            MVSNeRF~\cite{chen2021mvsnerf} & 0.676 & \textbf{0.826} & 0.858 & 0.821 & 0.634 & 0.642 & 0.921 & 0.820 \\
            GeoNeRF~\cite{johari2022geonerf} & \textbf{0.727} & 0.805 & 0.818 & 0.821 & 0.706 & 0.604 & 0.836 & 0.817 \\
            \midrule
            \textsc{Free-Editor} & 0.723 & 0.818 & \textbf{0.861} & \textbf{0.865} & \textbf{0.732} & \textbf{0.635} & \textbf{0.878} & \textbf{0.841} \\
            \bottomrule
            \end{tabular}}

            \scalebox{0.9}{
            \begin{tabular}{l|cccccccccc}
            \toprule
             & \multicolumn{8}{c}{LPIPS$\downarrow$} \\
            \cmidrule{2-9}
            &  Fern & Flower & Fortress & Horns & Leaves & Orchids & Room & T-Rex \\
            \midrule
            MVSNeRF~\cite{chen2021mvsnerf} & 0.262 & 0.225 & 0.210 & 0.281 & 0.325 & 0.298 & 0.206 & 0.234 \\
            GeoNeRF~\cite{johari2022geonerf} & \textbf{0.225} & 0.212 & 0.153 & 0.169 & \textbf{0.254} & 0.294 & 0.198 & 0.249 \\
            \midrule
            \textsc{Free-Editor} & 0.237 & \textbf{0.195} & \textbf{0.128} & \textbf{0.173} & 0.263 & \textbf{0.275} & \textbf{0.187} & \textbf{0.228} \\
            \bottomrule
            \end{tabular}}
    \end{center}
    % %\vspace{-2.5ex}
    \label{table:llfe_pert}
    %\vspace{-2ex}
    % %\vspace{-5.5ex}
\end{table*}
\subsubsection{Ray Transformer}
The ray transformer block integrates multi-headed self-attention and cross-attention layers with four heads. Each block maintains a dimensionality of $64$.  Consistent with ~\citet{vaswani2017attention, mildenhall2021nerf}, we transform low-dimensional coordinates into a higher-dimensional representation using Fourier components, selecting 10 frequencies for all experiments. The resulting view and position embeddings each have a dimension of $63$. 

\begin{figure}[thb]
    \vspace{-3mm}
    \centering
    \includegraphics[width=0.98\linewidth]{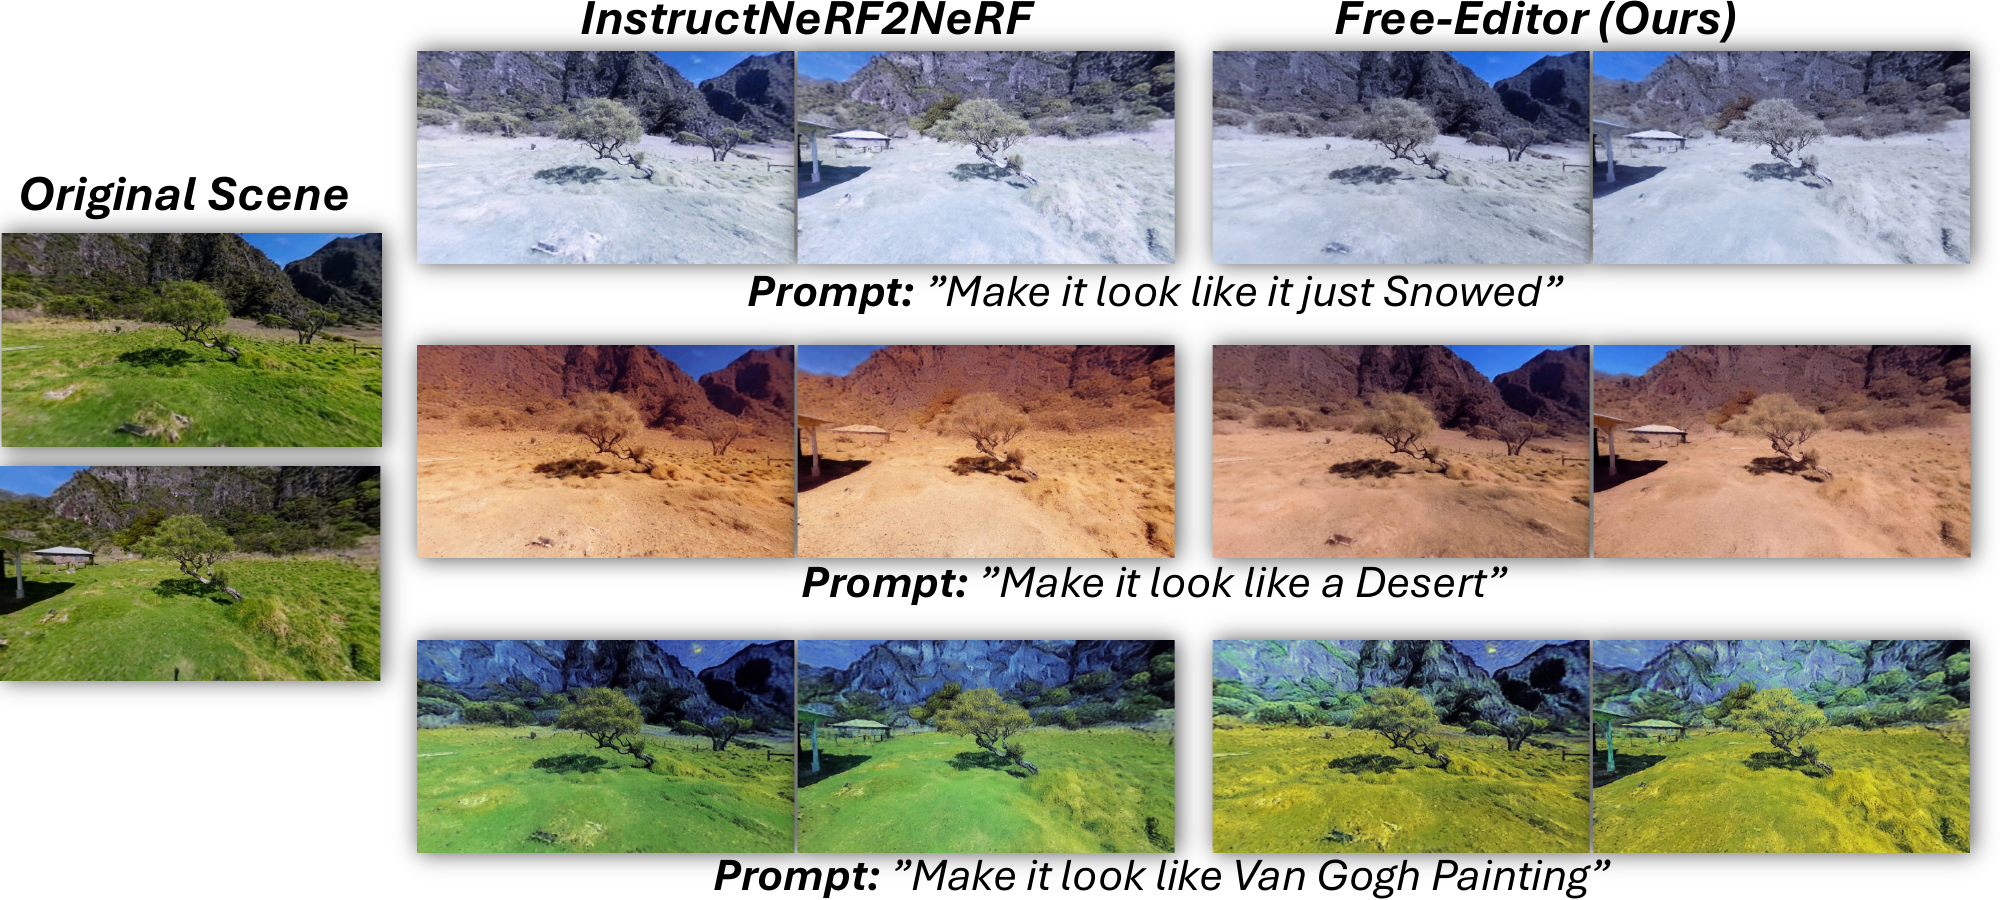}
    \vspace{-2.5mm}
    \caption{\footnotesize \textbf{Performance comparison of IN2N and Free-Editor on Large Outdoor Scene.} Our proposed approach demonstrates comparable editing results to IN2N across various text prompts. The overall advantage of Free-Editor is notable, particularly considering its 20$\times$ increase in speed compared to IN2N. Please zoom in for a better view.}
    \label{fig:large_scene}
    \vspace{-3.5mm}
\end{figure}
\subsection{Details of Training and Inference}\label{sec:training_and_inference}
% \textcolor{red}{Fix this and Write as much as possible }

% During training, we choose 12 starting view images from each scene and edit them using 6 different target captions. Therefore, there are . Each of these starting "Image-Caption" pairs is accompanied by an M number of unedited source-view images. 

During training, we choose different starting view images from each scene and edit them using 6 different target captions.  We use an Adam Optimizer for optimizing the model with learning rates of 2e-4 for the Edit Transformer, 1e-4 for the Epipolar transformer, and 5e-4 for the Ray Transformer. In addition, a batch size of 2048 rays has been employed for training. In every batch, we select rays from eight distinct scenes. Within each scene, we randomly sample rays from a singular image for training purposes. As for the loss coefficients, we consider 5e-4, 1e-3 and 1e-4 for  $\lambda_c,  \lambda_s, \text{and} \hspace{1mm} \lambda_e$, respectively. In our work, we calculate $\textit{L}_{con}$ only after 20K iterations. We employ the PyTorch framework~\cite{paszke2019pytorch} to implement our proposed method and train the model using 8 RTX 3090 NVIDIA GPUs for 4 days. For inference, a single RTX 3090 has been used.  We use a linear
learning rate warm-up for 5k iterations and cosine decay afterward. During training, we uniformly sample M from [8,12] while it is varied from 3 to 18 during inference. We recommend using $M=12$ considering the performance-computation trade-off. The number of sampled points along each ray ($N_P$) is set to be 64.  In addition to PSNR and CTDS, we employ quantitative evaluation metrics such as SSIM (structural similarity index measure), and LPIPS (learned perceptual image patch similarity).   

Note that, in our work, we select spatial points and project them onto the source views to obtain their respective colors and image characteristics. However, the projected pixel of a sample can fall outside the image plane. In such instances, we exclude the corresponding source view for that sample. If a point isn't projected onto the image plane of any source view, we assign a volume density of zero to that point. If fewer than three samples on a ray possess valid density values, we disregard that ray in the loss function during training.

\section{User Study Details}\label{sec:user_study}
We invited a total of 30 participants (21 Male, 9 Female, aged 20 to 50) for this particular study. Every user views videos or frames generated using different techniques and then chooses their preferred option based on three specific factors: 3D consistency, content preservation, and fidelity to the text description. The first factor indicates the degree to which the 3D scenes 
maintain consistency across different views.  Content preservation describes the model's effectiveness in precisely editing the targeted object whereas we use text fidelity to describe the capability of the model to generate an edited image that accurately reflects the text condition. We used a total of 10 scenes and 8 different prompts for this experiment and asked the user to rate the edited images based on the factors described above.   

\section{Additional Results}\label{sec:add_results}
In this section, we provide both qualitative and quantitative results.
\subsection{Qualitative Results}\label{sec:qual}
We present additional results for style transfer as well as text-driven editing. In Figure~\ref{fig:text_to_3D_1}, it can be observed that \textsc{Free-Editor} successfully learns how to transfer different style information from the starting view to novel views. This type of transfer enables us to obtain 3D-edited scenes. Note that, the background in target views may be affected by the editing which should not take place in general. This is a challenging issue to tackle as no further training is involved. However, one should obtain better performance with additional training on a larger training dataset.  

\subsubsection{Additional Comparison with IN2N} In Figure~\ref{fig:large_scene}, we present the editing results on large-scale outdoor scenes for both IN2N and Free-Editor. We apply three different prompts to demonstrate the style transfer capabilities of both methods. Similar to “Lego with Van Gogh" in the paper, Free-Editor is able to perform effective style transfer (not just tone change). For bear and portrait, the side-by-side comparison can be observed in Figure~\ref{fig:bear_portrait}. Our proposed approach accurately produces the content provided in the text prompts, while effectively preserving the consistency of the input objects. 
% We will include these additional qualitative results, their corresponding videos, and quantitative results (due to space constraints of the rebuttal) in the final version of our paper.
\begin{figure}[h]
    \vspace{-3mm}
    \centering
    \includegraphics[width=0.95\linewidth]{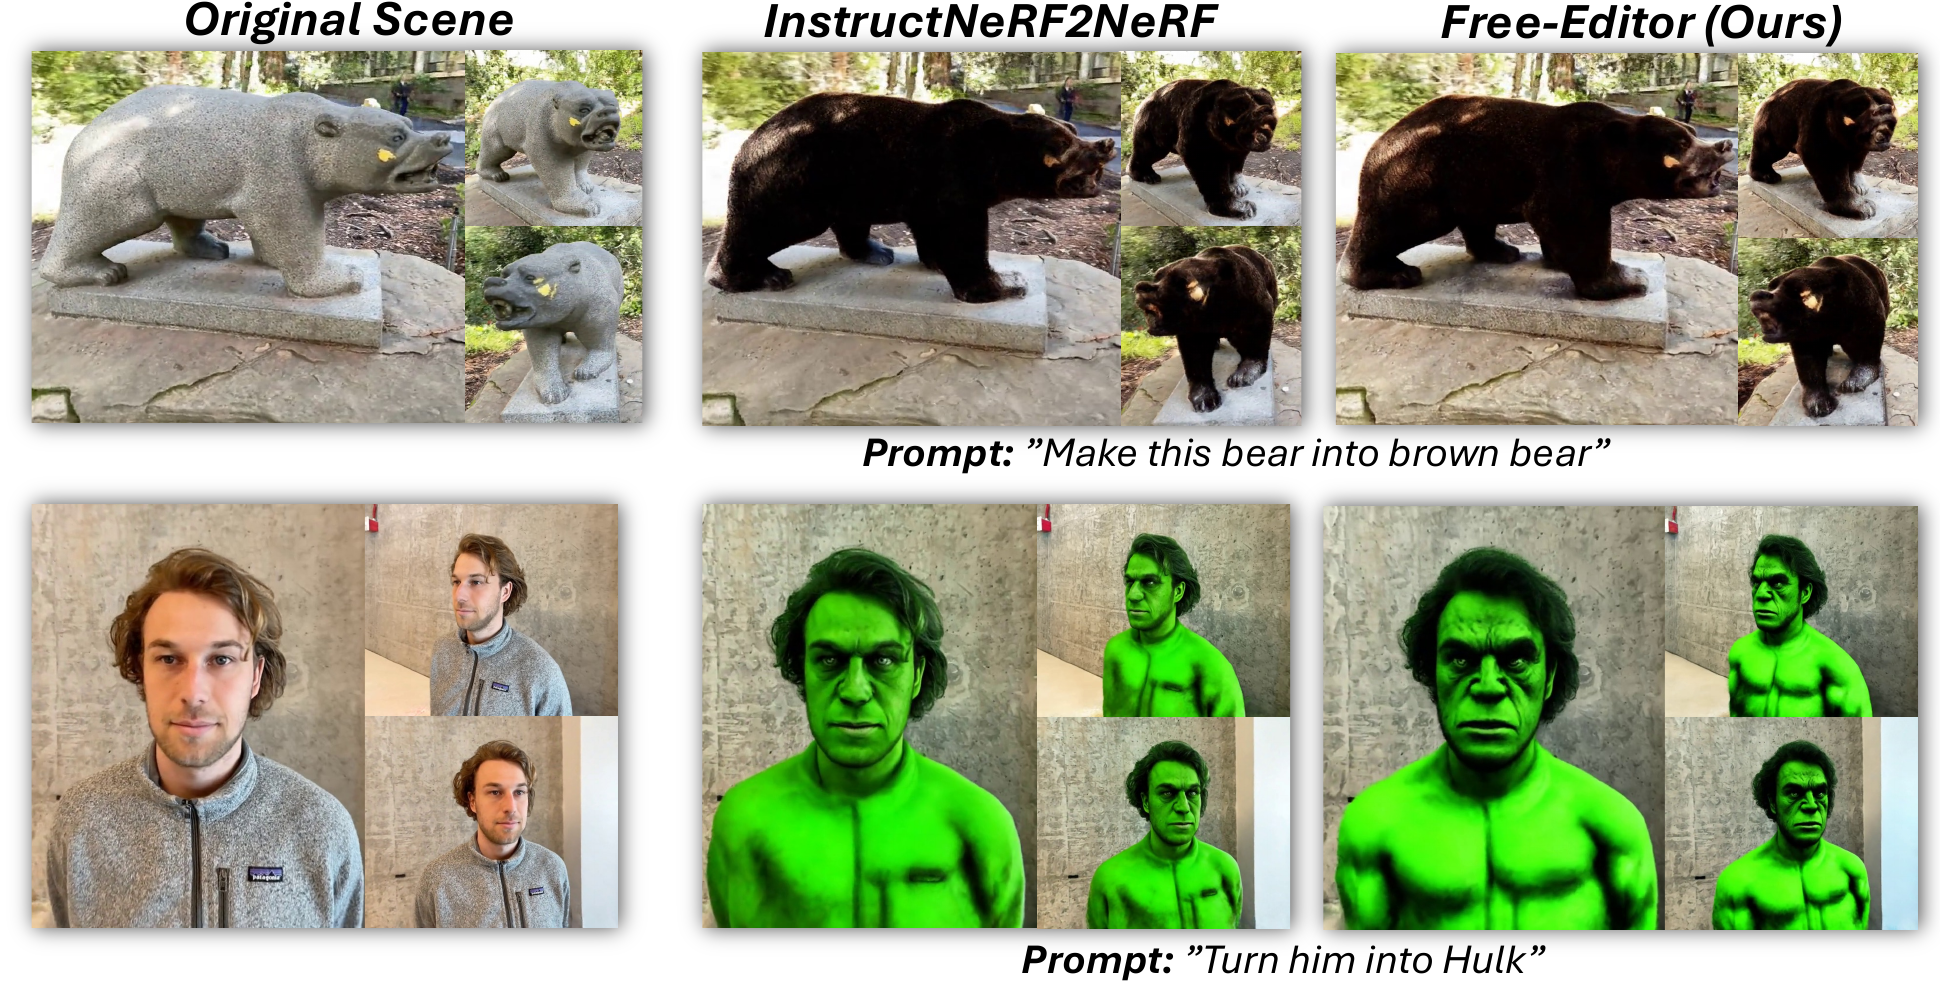}
    \vspace{-2.5mm}
    \caption{\footnotesize \textbf{Additional Comparison on Bear and Portrait.} The performance of Free-Editor is consistent across both the scenes. }
    \label{fig:bear_portrait}
    \vspace{-4mm}
\end{figure}

\subsection{Quantitative Results}\label{sec:quant}
In Table~\ref{table:llfe_original}, we present the per-scene metrics for the real forward-facing LLFF dataset. Note that, our method is specifically developed for 3D scene editing tasks. Unlike other generalizable methods, we are focusing on the content of a single (starting) view heavily while combining features from other source views too. This may cause \textsc{Free-Editor} to perform poorly in the case of regular LLFF where we do not perform any editing. However, the main objective of this work is successfully obtained as shown by the results in Table~\ref{table:llfe_pert}. When we edit the reference view images, SOTA generalizable methods severely underperform as compared to their unedited synthesis results (in Table~\ref{table:llfe_original}).

\section{Discussion}\label{sec:need_for_free_editor}
Since we are using the Gen-NeRF, it may be natural to ask whether we can obtain the same type of abilities as Free-Editor with very minor modifications. We argue that a simple altering in conventional Generalized NeRF (Gen-NeRF) will not lead to Free-Editor for the following reasons: \textcolor{orange}{i)} In our work, we aim to address the issue of \emph{viewpoint inconsistency} in current T2I models. If we followed any of the currently available Gen-NeRF methods, it would require us to edit most (if not all) training images which would lead us to the same inconsistency issue; \textcolor{orange}{ii)} As a solution to this issue, we \emph{propose to edit only a single view (starting view)} instead of all training views. Even if we were to edit a single view for current Gen-NeRF methods, none of them can accommodate the setup of learning from one edited starting view and transferring these edits to other views;
\textcolor{orange}{iii)} To solve this, we introduce a \emph{novel Edit Transformer (ET)} which may seem trivial but plays a significant role in achieving the overall objective;  \textcolor{orange}{iv)} In addition, it is required to use the \emph{proposed loss functions} to achieve accurate editing effects. Without taking these factors into account, one cannot simply obtain viewpoint-consistent 3D scene editing through minor modifications to current Gen-NeRF methods. Therefore, we need a specialized technique that can perform Text-based 3D Scene Editing with in a consistent fashion and diverse edting capabilities.
